# Supplementary material for: STanH : Parametric Quantization for Variable Rate Learned Image Compression
Source: arXiv:2410.00557 source file (2024-10-12)
Supplement: Supplementary file 1 [file 7_appendix.tex]

\section{Additional material}
%In this section, we present some additional data and results that we omitted in the main work due to space constraints. These results do not contribute to any theoretical message in our study; rather, they aim to provide a more comprehensive view of the outcomes obtained with our method.

\subsection{Hyper-parameter used for different number of anchors}\label{lambdas}

Tab. \ref{tab_lambdas} reports different values of $\lambda$ used for training our \stanh in \emph{Zou22}, in the case of a number of anchors different than three.
We evenly distributed the anchors across the RD range, ensuring that the chosen $\lambda$'s closely aligned with those used in the reference works we compared to.

\begin{table}[!h]
\centering
\small
 \caption{Values of $\lambda$ used for both training anchors and their derivations, considering \emph{Zou22} as reference model. $A_{:}$ represents a vector related to all anchors, while $D_{i,:}$ represents all the derivations obtained from the $i$-th anchor.}
\resizebox{\columnwidth}{!}{\begin{tabular}{ccc}
  \toprule
  \textbf{\emph{\# Anchors}} & \multicolumn{1}{c}{$\lambda$ used for anchors} & \multicolumn{1}{c}{$\lambda$ used for derivations.} \\
  \midrule
  \emph{6}&  $A_{:} = \left \{0.0483, 0.025, 0.010, 0.0067, 0.0025, 0.0018 \right\}$ & $\emptyset$ \\
  \emph{5}& $A_{:} = \left \{0.0483, 0.025, 0.010, 0.0067, 0.0025 \right\}$ & $D_{5,1} = \left \{ 0.0012 \right\}$ \\
  \emph{4}& $A_{:} = \left \{0.0483, 0.025, 0.010,  0.0025 \right\}$ &  $D_{4,1} = \left \{ 0.0012 \right\}$,  $D_{3,1} = \left \{ 0.0060 \right\}$   \\
  \emph{2} &  $A_{:} = \left \{0.0483, 0.010 \right\}$&  $D_{2,:} = \left \{ 0.0022, 0.0060 \right\}$,  $D_{1,:} = \left \{ 0.022, 0.015 \right\}$  \\
  \emph{1}& $A_{:} =  (0.0483)$ & $D_{1,:} \left\{0.018, 0.010, 0.0067, 0.0025, 0.0009\right\}$  \\
  \bottomrule
\end{tabular}}\label{tab_lambdas}
\end{table}

\subsection{Analysis of \stanh  quantizer} \label{functioning}

Fig.\ref{anchor} shows the reconstruction length of the central quantization levels related to $\mathbf{\hat{y}}$ formed during training for \emph{Zou22} taking $A_{1}$ as anchor and three corresponding derivations ($D_{11},D_{12},D_{13}$).
We show only central quantization levels because they contain most of the information and vary the most between the anchor and the derivations. The plot shows the length of the quantization intervals trained with different values of $\lambda$ (the horizontal axis reports the corresponding reconstruction levels, mapped on integers for simplicity.
%), while on the vertical axis we report their lengths for different quality levels;
The major differences are visible on the central levels (close to zero) 
where the lowest quality model has larger quantization intervals.
These results confirm the intuition that using \stanh we partially decouple image transformation from quantization: in particular fine-tuning only the parametric quantizer we get larger quantization steps yielding a coarser representation of the latent space.
%(almost doubling the quantization step for the lowest quality ones. 
%From the figure, it is understood how, when one aims to optimize \emph{Stanh} at a lower quality, both levels zero and one levels become progressively larger, thus encompassing more values during the quantization process and making it less refined. 
%The refining process also affects the other levels, albeit to a lesser extent; generally, the rule still applies that lower quality leads to a longer average length compared to the starting anchor.

\begin{figure}[h!]
%\begin{minipage}[b]{1.0\linewidth} 
  \centering
 \includegraphics[width=0.5\columnwidth]{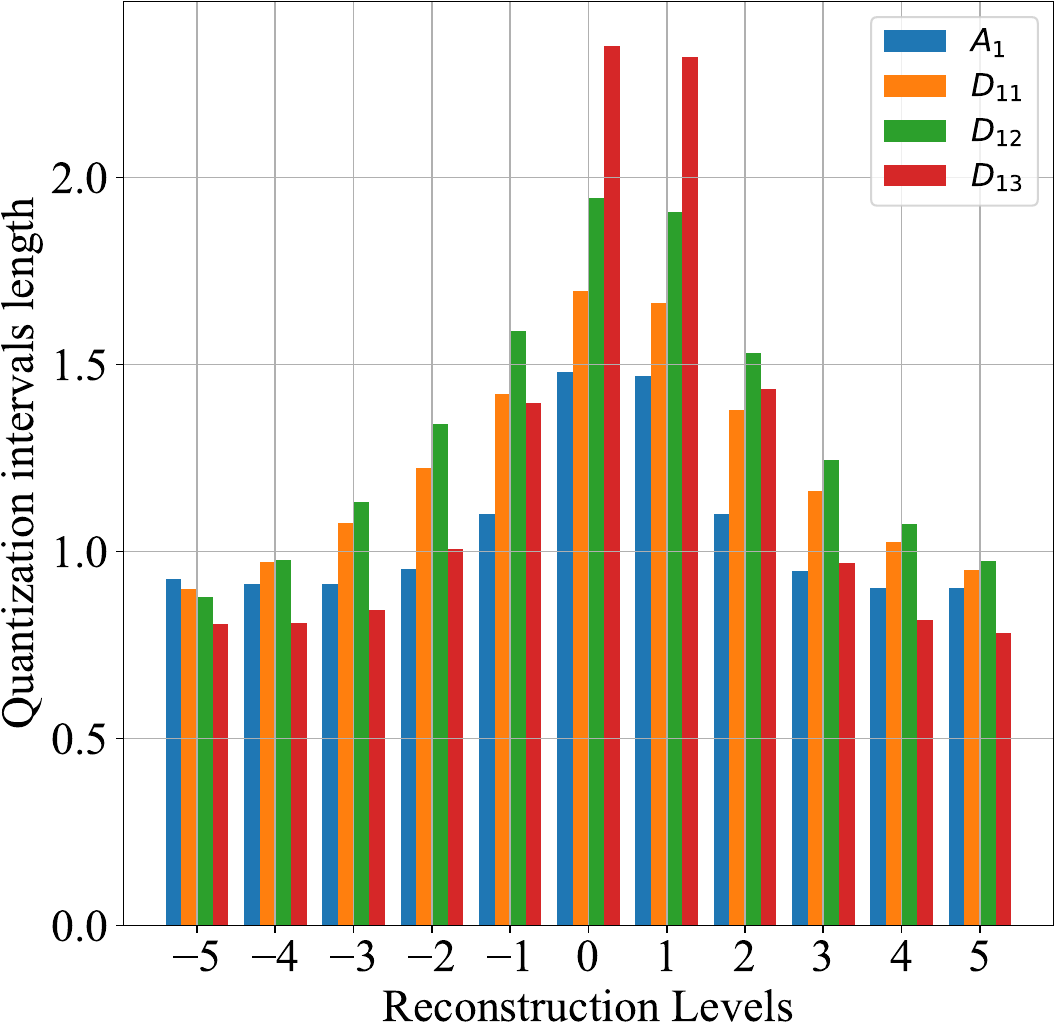}
 % \vspace{0.1cm}
  \caption{Distribution of Length of the quantization intervals for different qualities, taking \emph{Zou22} as Reference, considering derivations obtained from the highest rate anchor $A_{1}$} 
  \label{anchor}

\end{figure}

\subsection{Rate/MS-SSIM  Performance}
In addition to PSNR, we also analyze the MS-SSIM measure for different reference models (for conciseness in the main paper we only show the results obtained on Kodak dataset).  Fig. \ref{mssim_others} shows the MS-SSIM for the datasets not considered in the main work.

\subsection{\stanh vs. custom uniform quantization}
We compare \stanh with respect to manually adjusting the quantization step in the uniform quantization to obtain different qualities using the same latent representation. It is possible to observe that using handcrafted quantization steps, as we move away from the anchor (stars in the figure), we get a performance impairment with respect to \stanh; despite the fact it would be possible to obtain decent results with this approach, we show how a non-uniform quantizer like \stanh can make the architecture more robust and more resistant to rate-variability, obtaining a BD-Rate of -4.09 dB (using derivations with manual steps as reference).

\begin{figure}[h!]
%\begin{minipage}[b]{1.0\linewidth} 
  \centering
 \includegraphics[width=0.65\columnwidth]{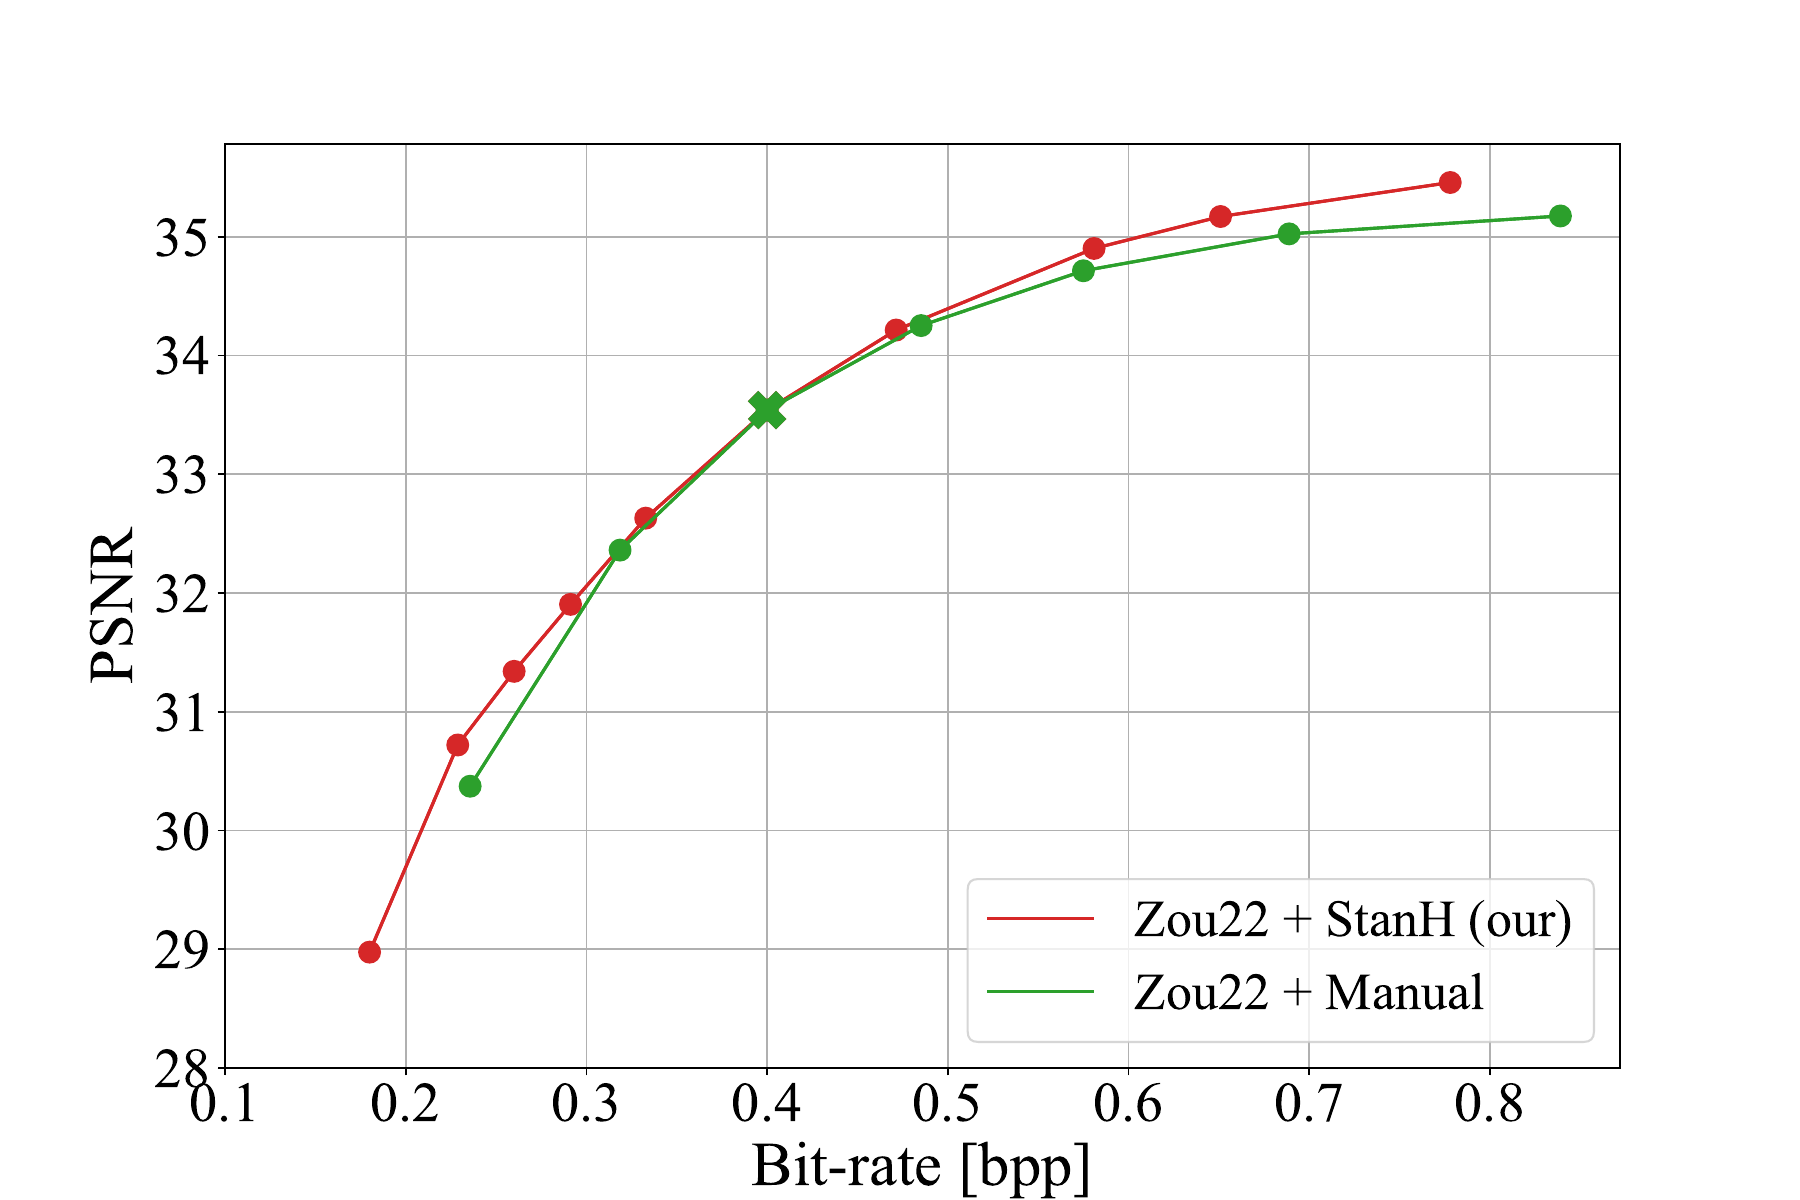}
 % \vspace{0.1cm}
  \caption{ Comparison between Proposed \stanh (red line) and manually adjusting the quantization step (green line)}
  \label{recostruct-cheng}
%\end{minipage}
\end{figure}

\subsection{Visual quality}
To prove the efficacy of our \emph{Stanh} module in terms of visual quality, in Figs.\ref{recostruct-cheng},\ref{recostruct-xie},\ref{recostruct-zou}) we report three reconstruction examples from the Kodak dataset, one for each reference models.
In particular, for each image we consider an anchor and a derivation, showing that the difference in performance with respect to reference models (and with VTM) is almost imperceptible at the human eye.
Other reconstructions from the Kodak dataset are available at \href{https://drive.google.com/drive/folders/18IkZvLhzFV8HUvNE9PYkeaaF4XDuGypQ?usp=drive_link}{https://drive.google.com/drive/reconstructions}

\begin{figure*}[!h]
  \centering

  \begin{subfigure}{0.3\textwidth}
    \centering
    \includegraphics[width=\textwidth]{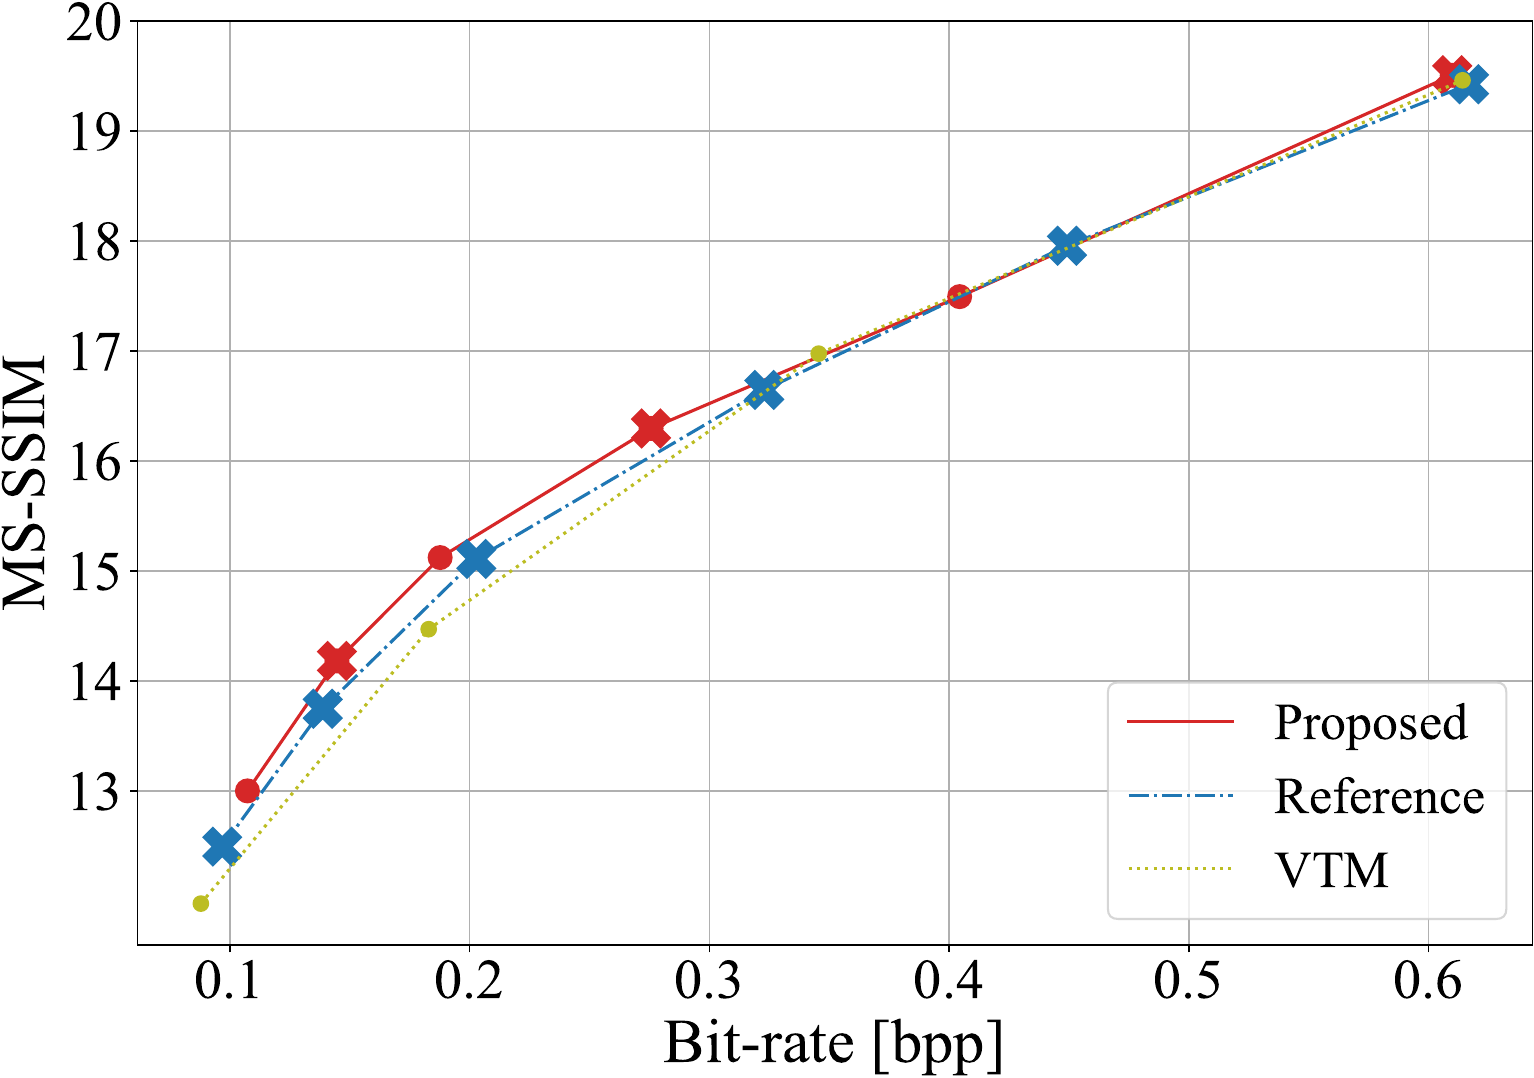}
    \caption{\emph{Cheng20}}
    \label{6aa}
  \end{subfigure}
  \hfill
  \begin{subfigure}{0.3\textwidth}
    \centering
    \includegraphics[width=\textwidth]{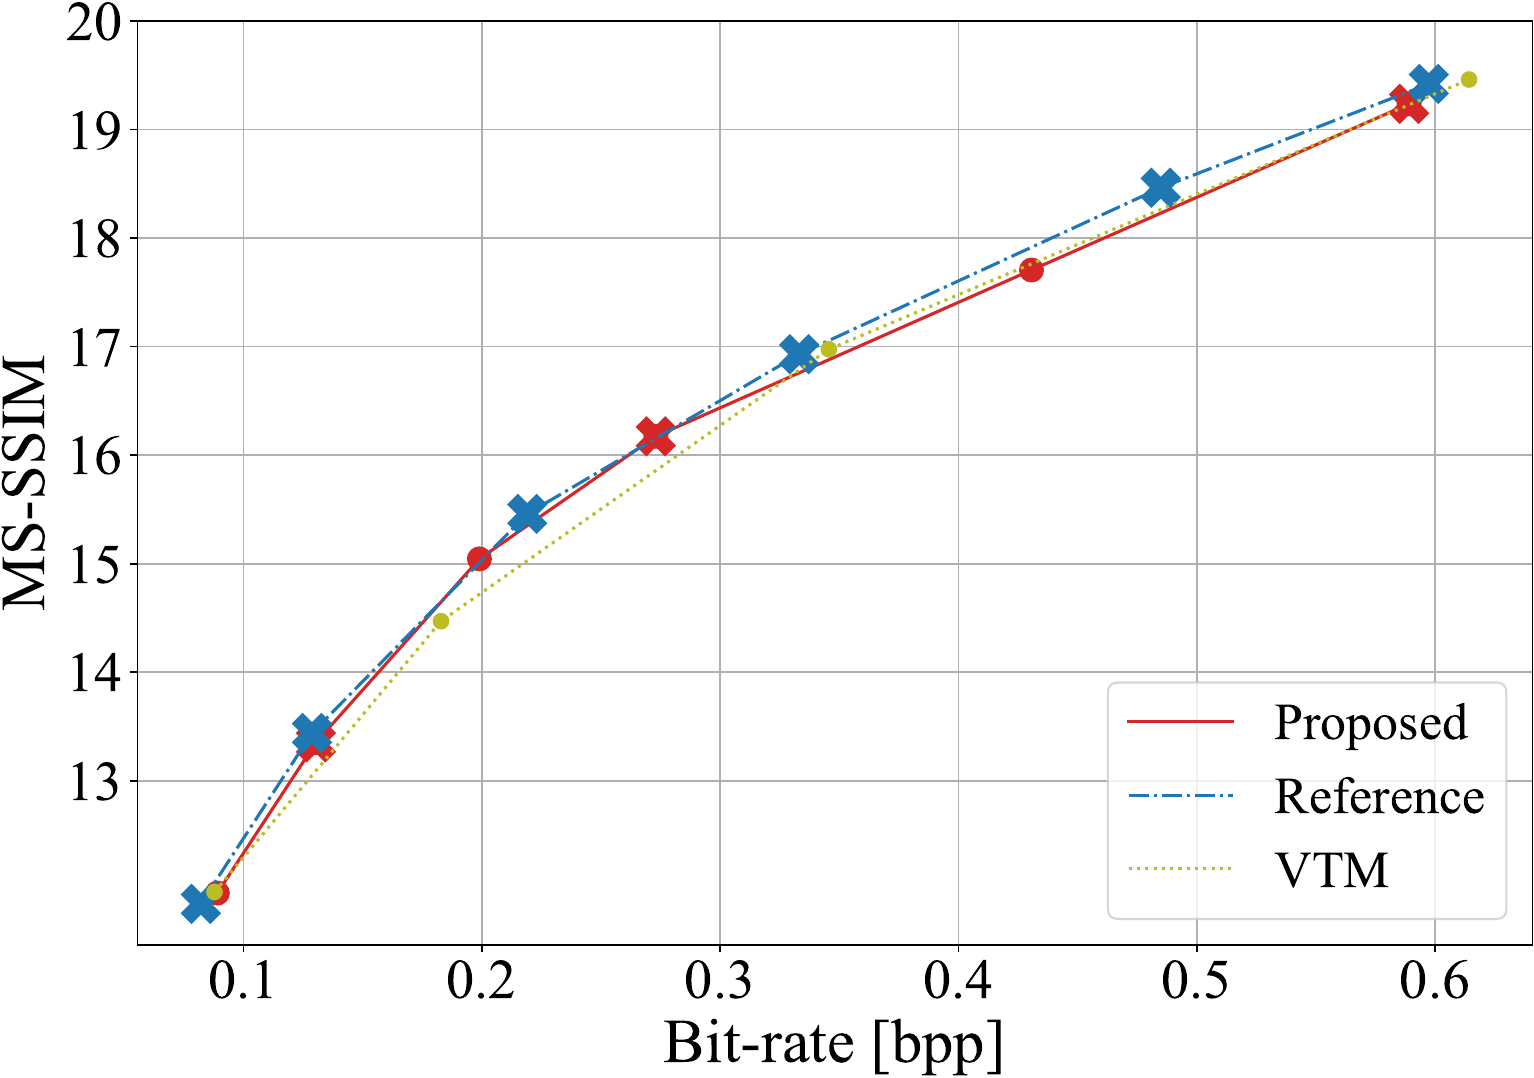}
    \caption{\emph{Xie21}}
    \label{3aa}
  \end{subfigure}
  \hfill
  \begin{subfigure}{0.3\textwidth}
    \centering
    \includegraphics[width=\textwidth]{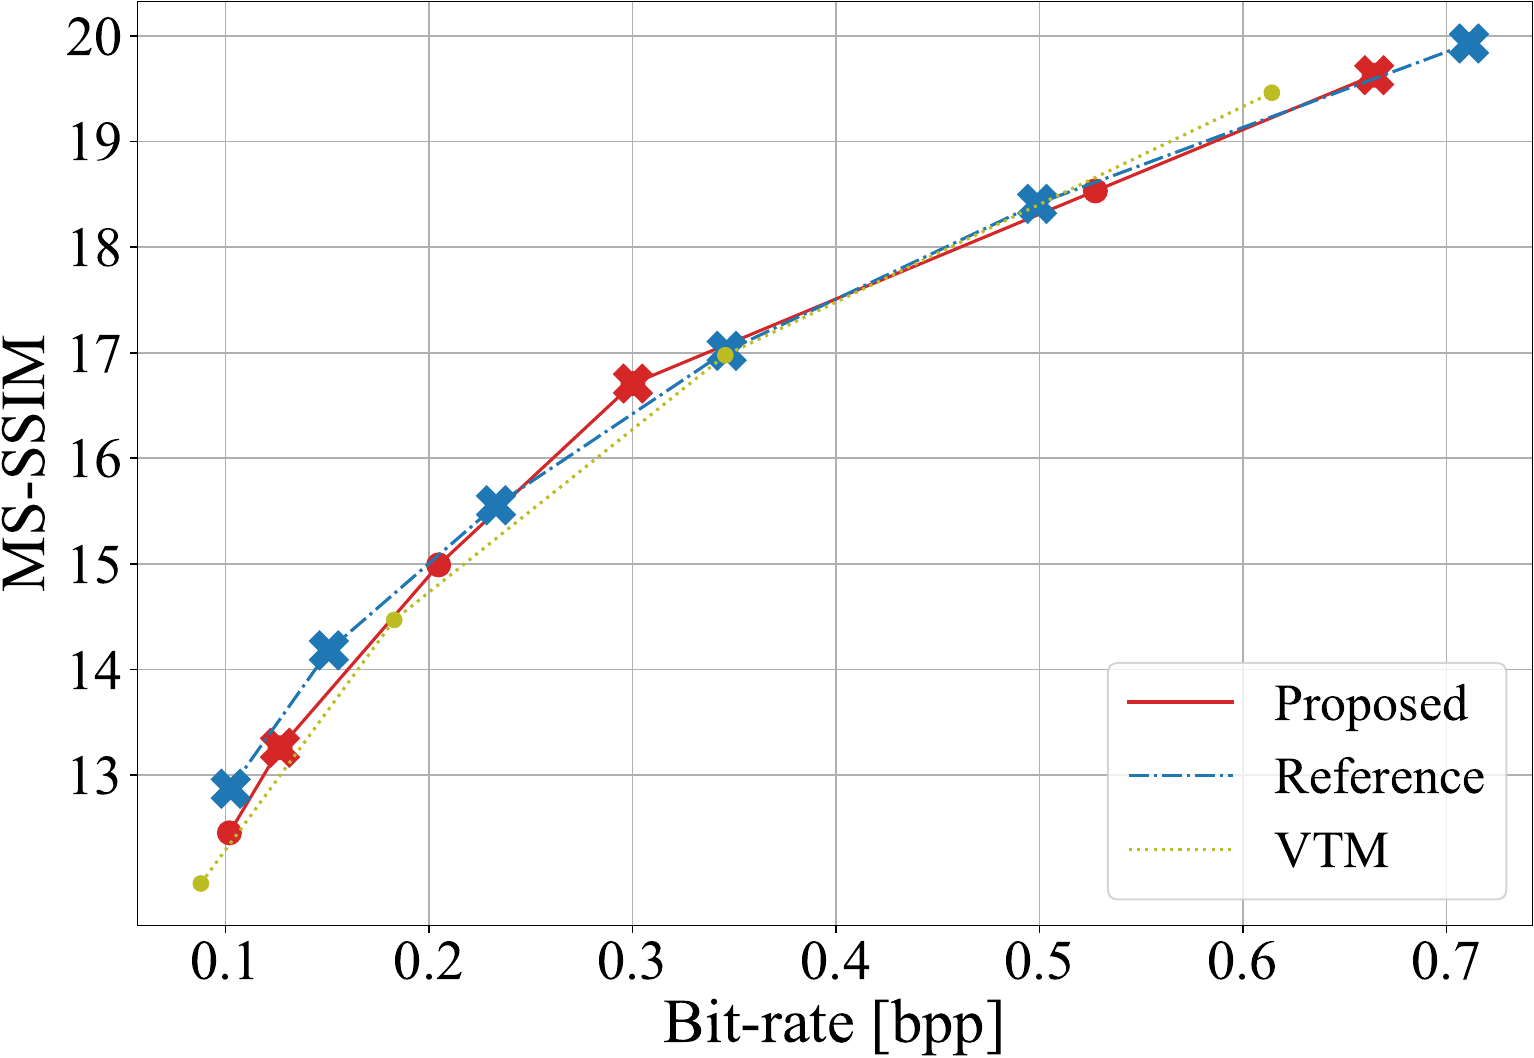}
    \caption{\emph{Zou22}}
    \label{4as}
  \end{subfigure}

  \vspace{\baselineskip}

  \begin{subfigure}{0.3\textwidth}
    \centering
    \includegraphics[width=\textwidth]{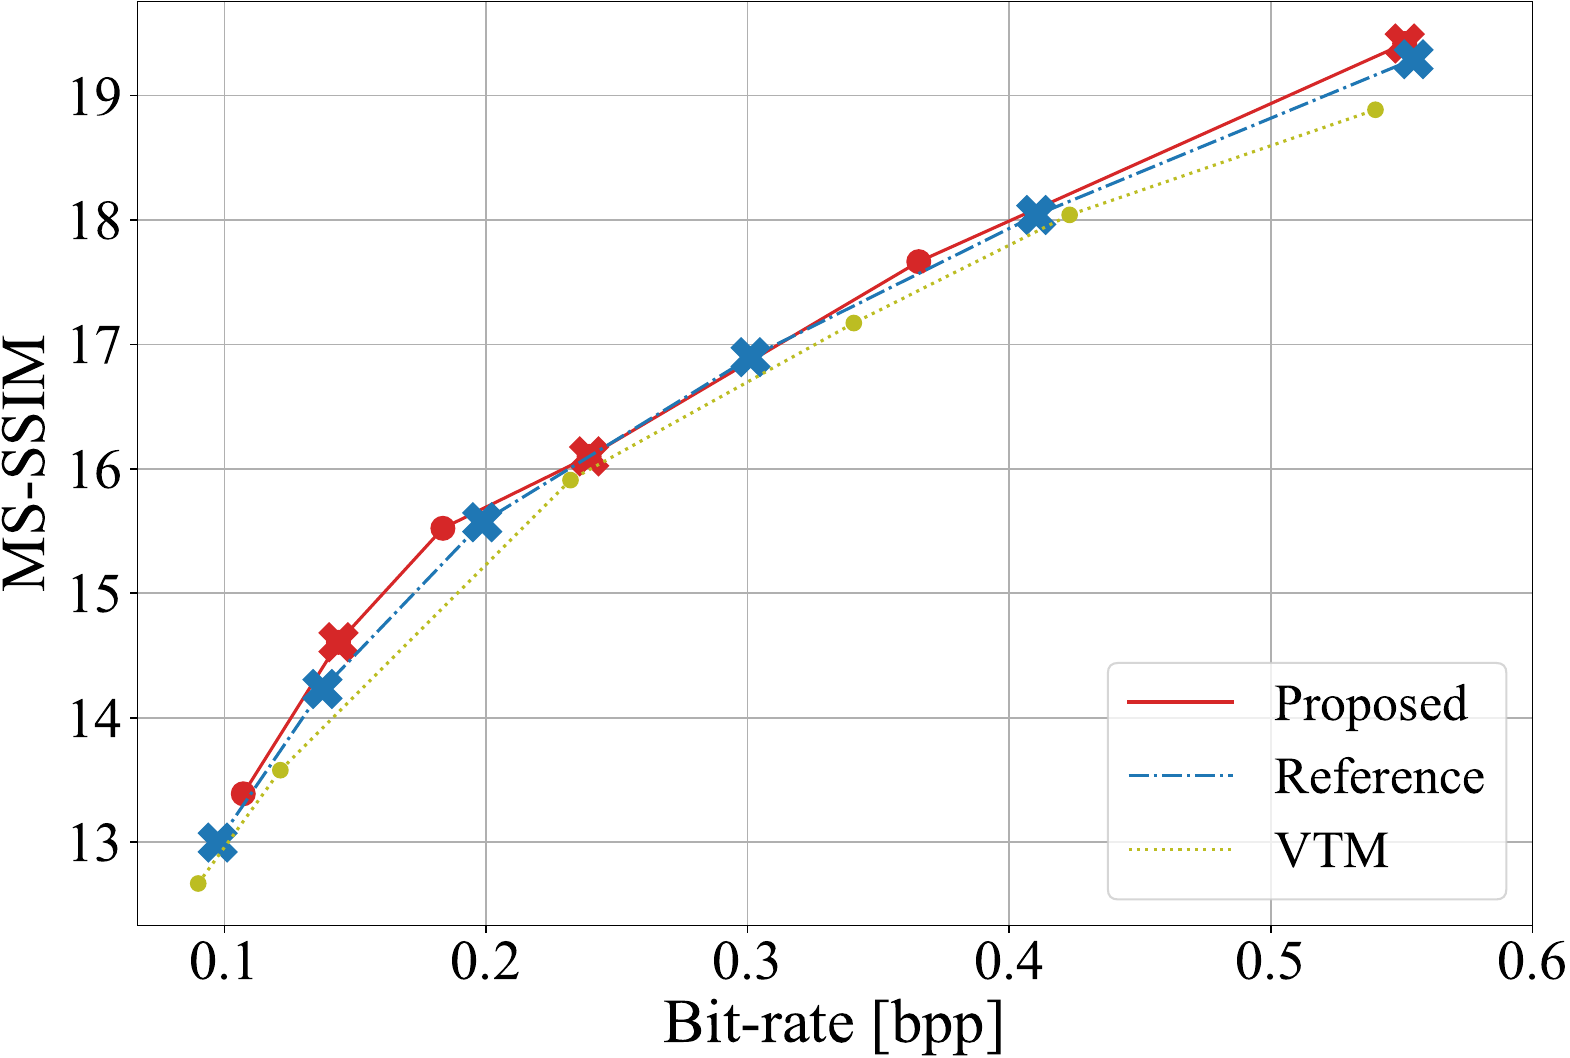}
    \caption{\emph{Cheng20}}
    \label{3a}
  \end{subfigure}
  \hfill
  \begin{subfigure}{0.3\textwidth}
    \centering
    \includegraphics[width=\textwidth]{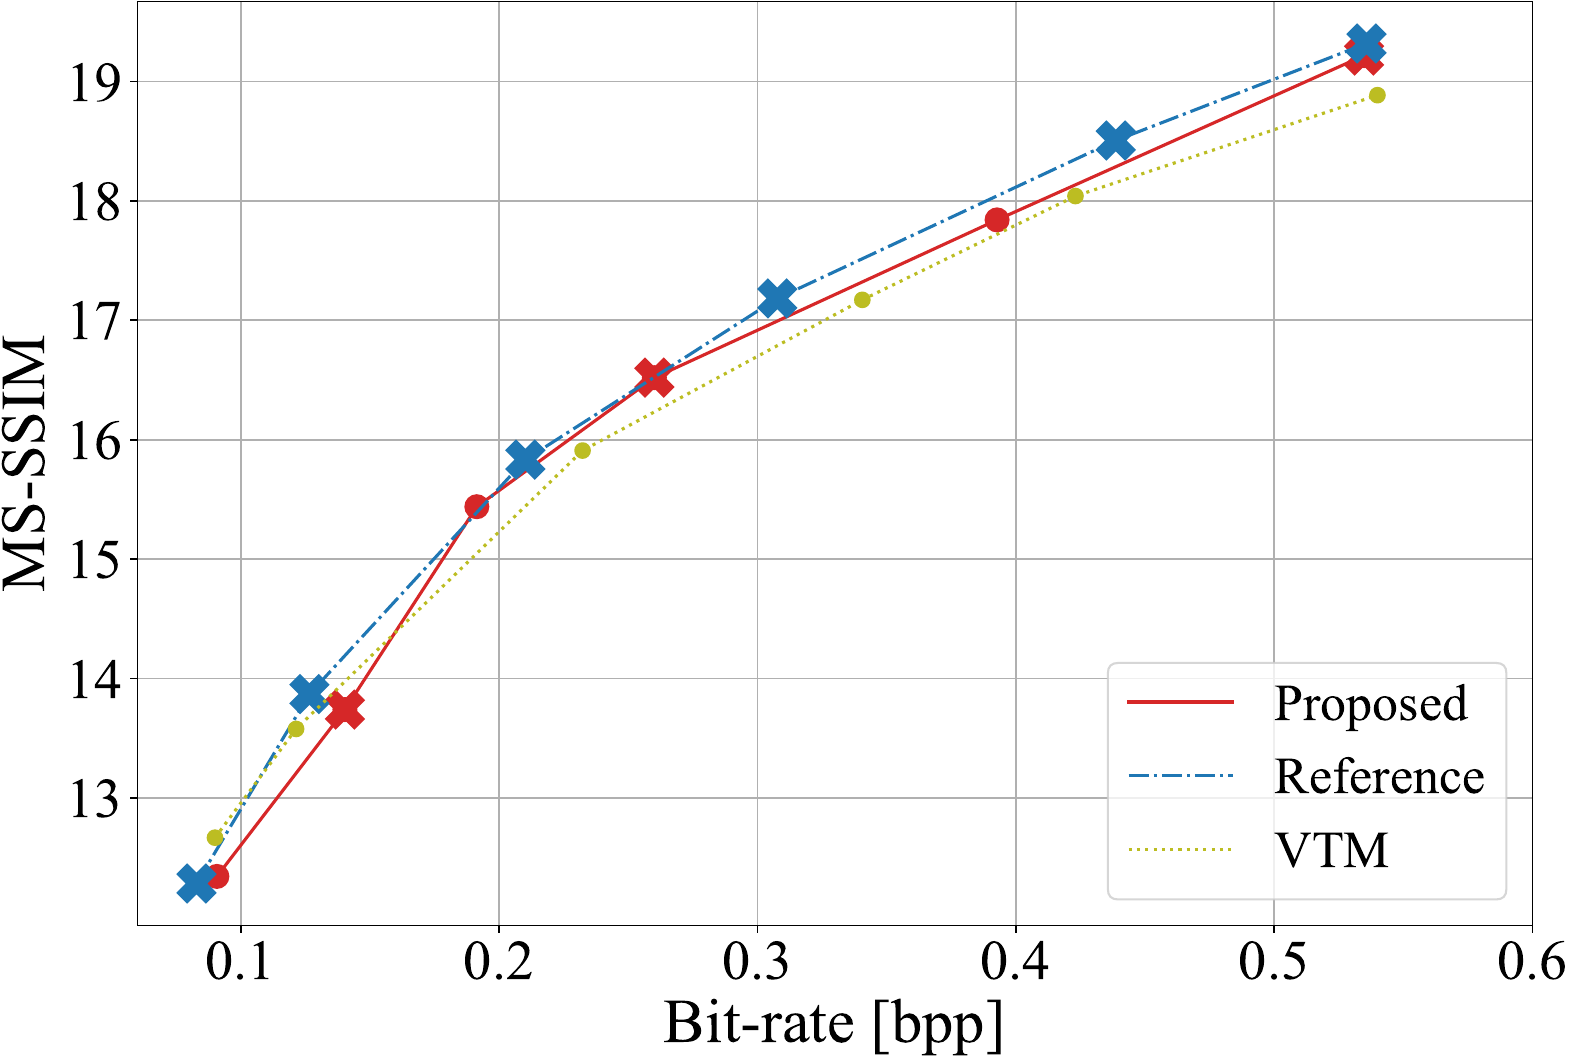}
    \caption{\emph{Xie21}}
    \label{2a}
  \end{subfigure}
  \hfill
  \begin{subfigure}{0.3\textwidth}
    \centering
    \includegraphics[width=\textwidth]{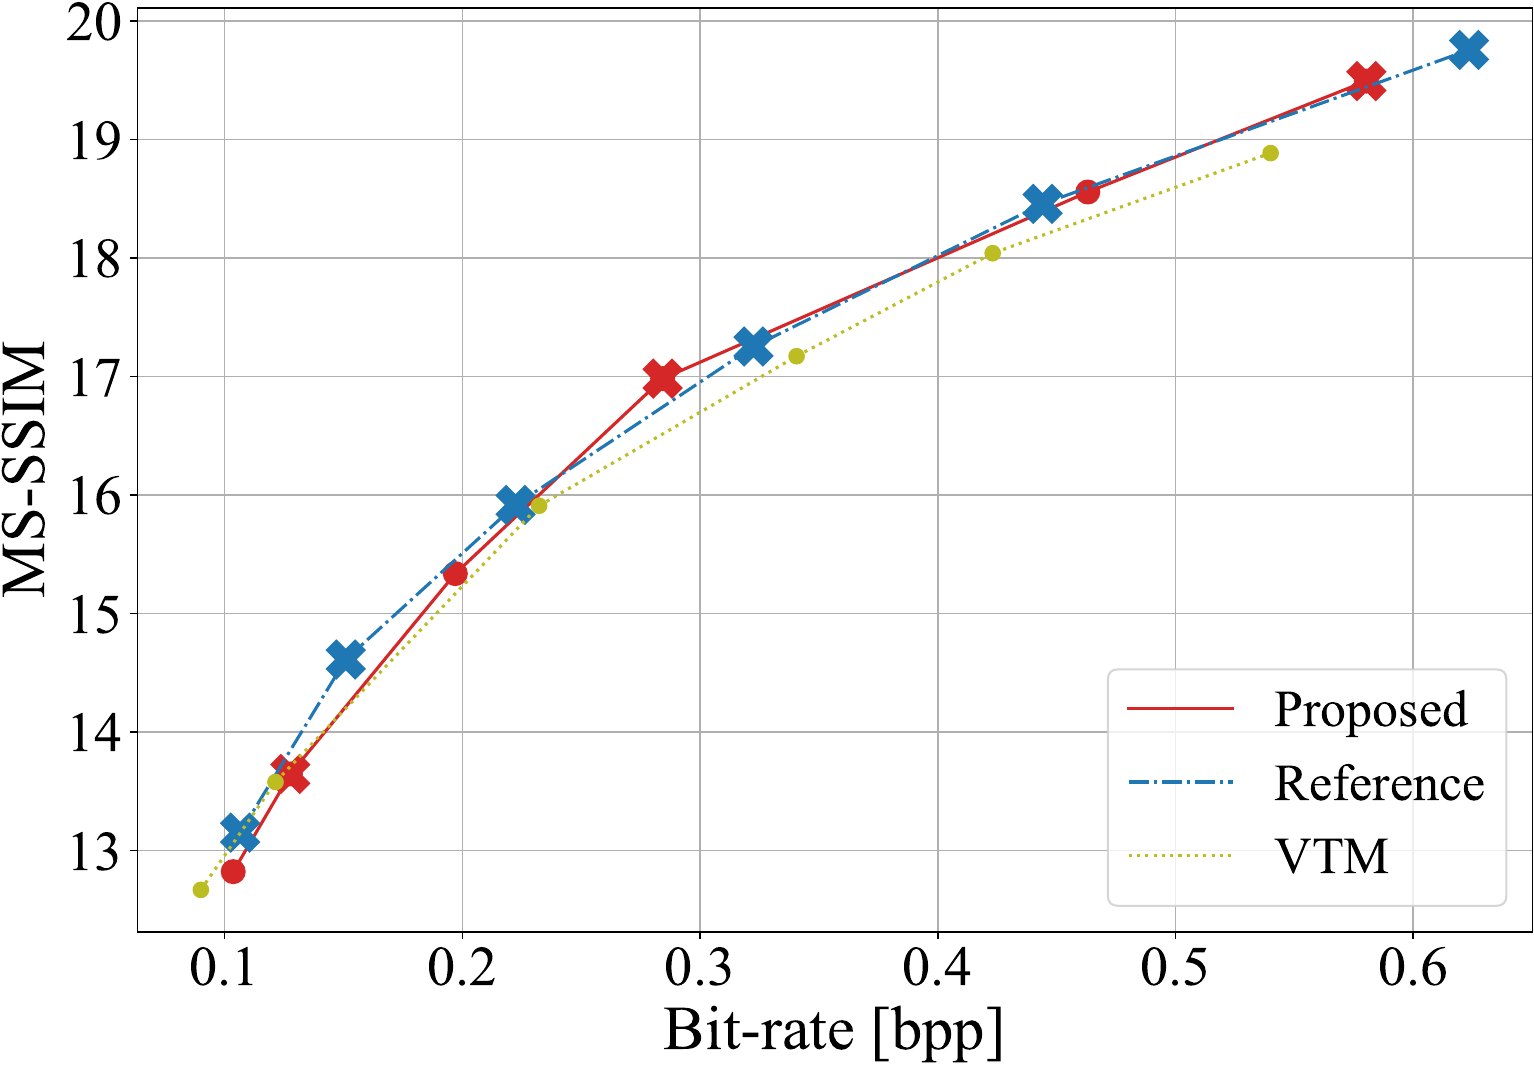}
    \caption{\emph{Zou22}}
    \label{1a}
  \end{subfigure}

  \caption{Rate/MS-SSIM  for the proposed Stanh-based method and relative reference for CLIC (top row) and Tecnik (bottom row) datasets and for 3 anchors.}

  \label{mssim_others}
\end{figure*}

\begin{figure*}[h!]
%\begin{minipage}[b]{1.0\linewidth} 
  \centering
 \includegraphics[width=\textwidth]{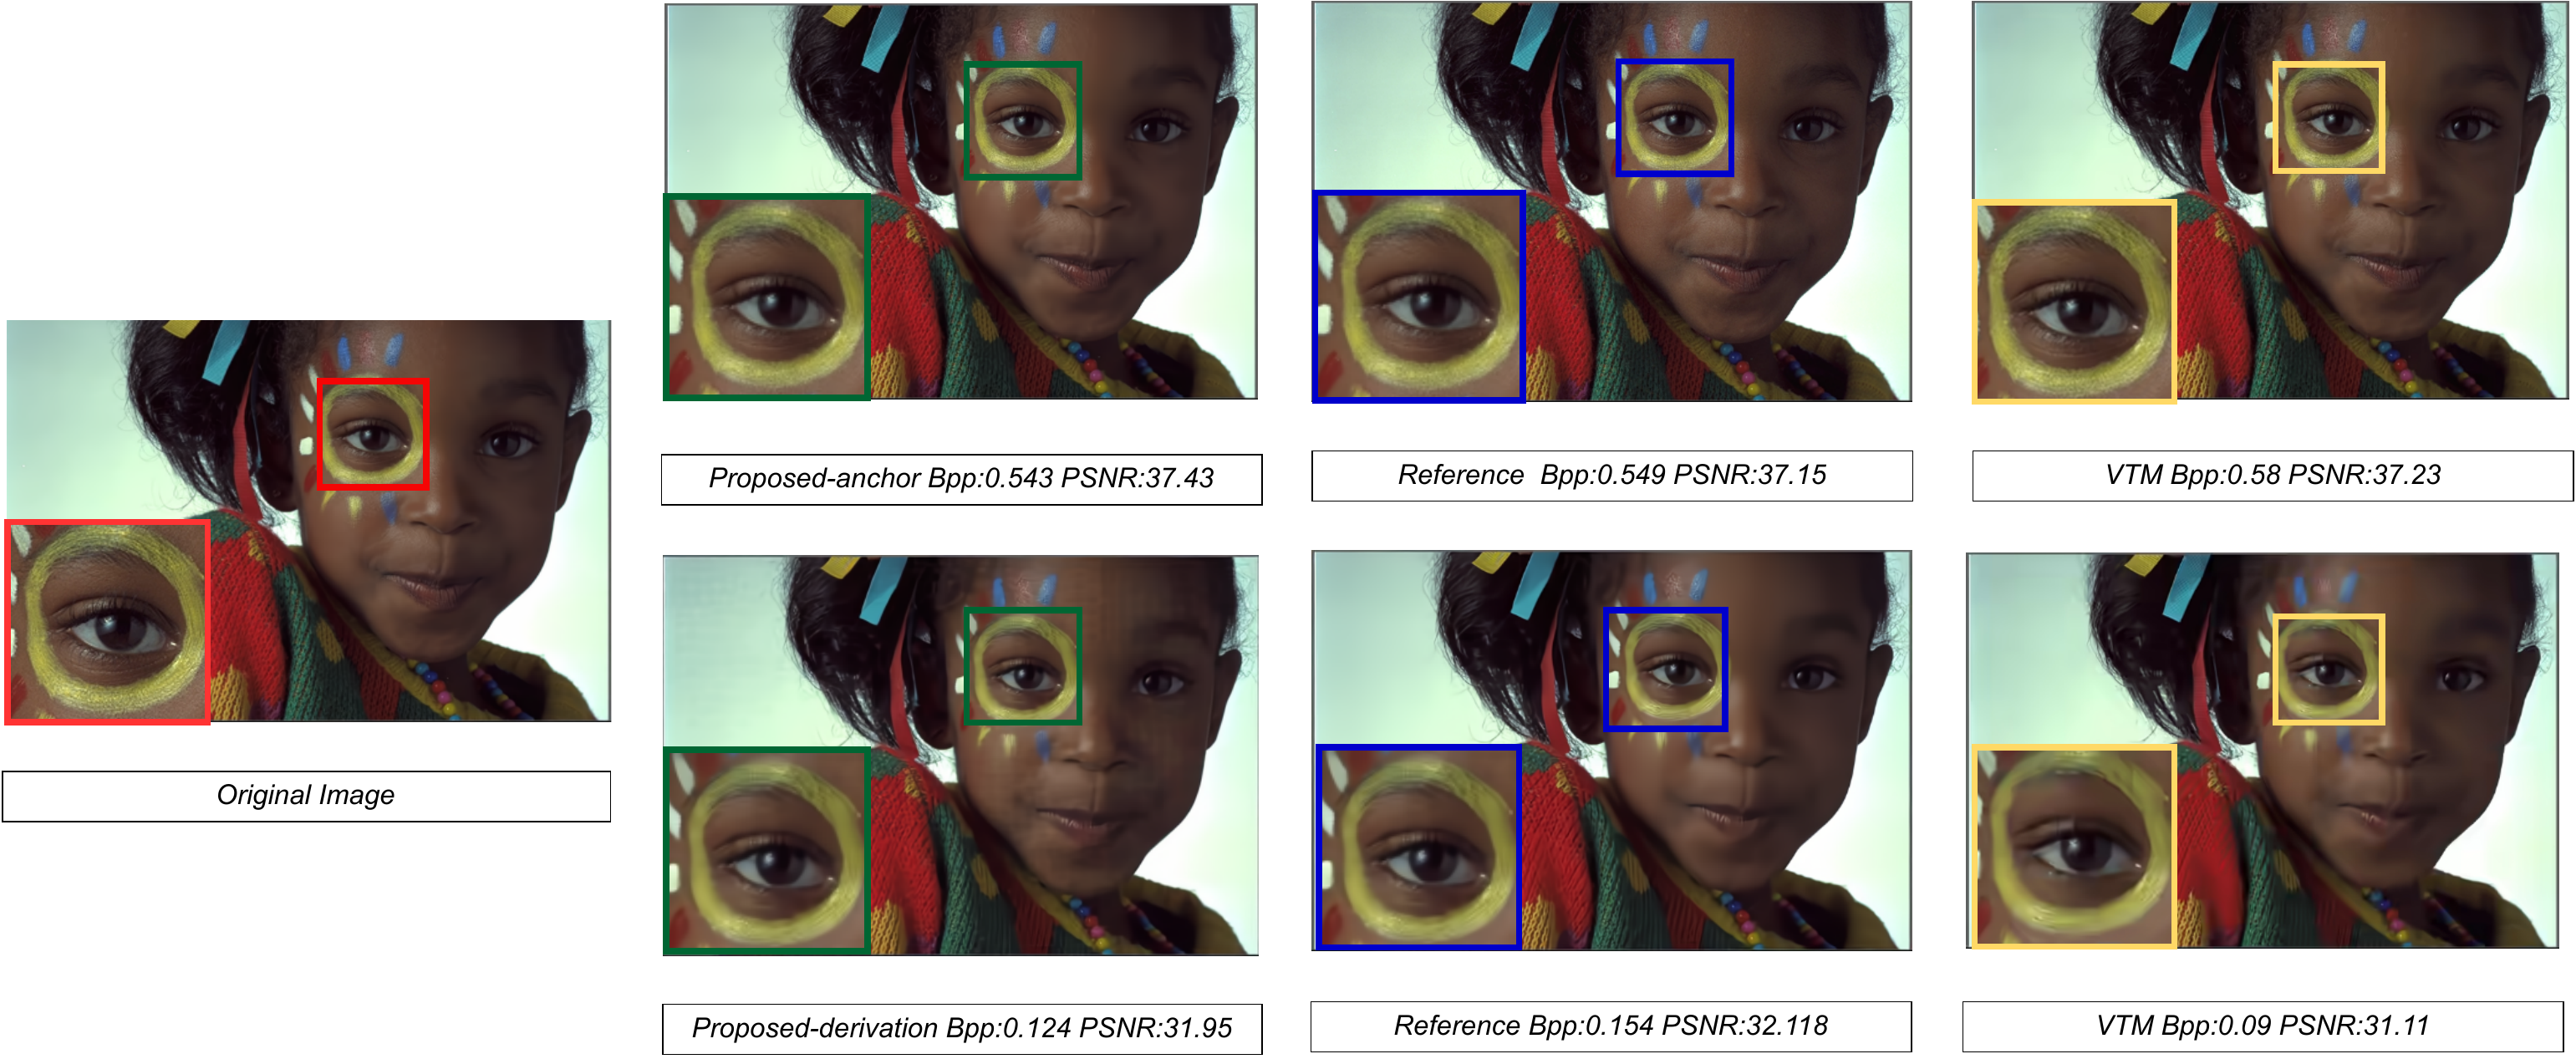}
 % \vspace{0.1cm}
  \caption{Reconstruction of \emph{Kodim15} using \emph{Cheng20} as reference. First row: Original image. Second Row: Comparison exploiting anchor model ($A_{1}$) Third Row: comparison exploiting Derivation model ($D_{21}$). Regarding reference, the closest one has been chosen. }
  \label{recostruct-cheng}
%\end{minipage}
\end{figure*}

\begin{figure*}[h!]
%\begin{minipage}[b]{1.0\linewidth} 
  \centering
 \includegraphics[width=\textwidth]{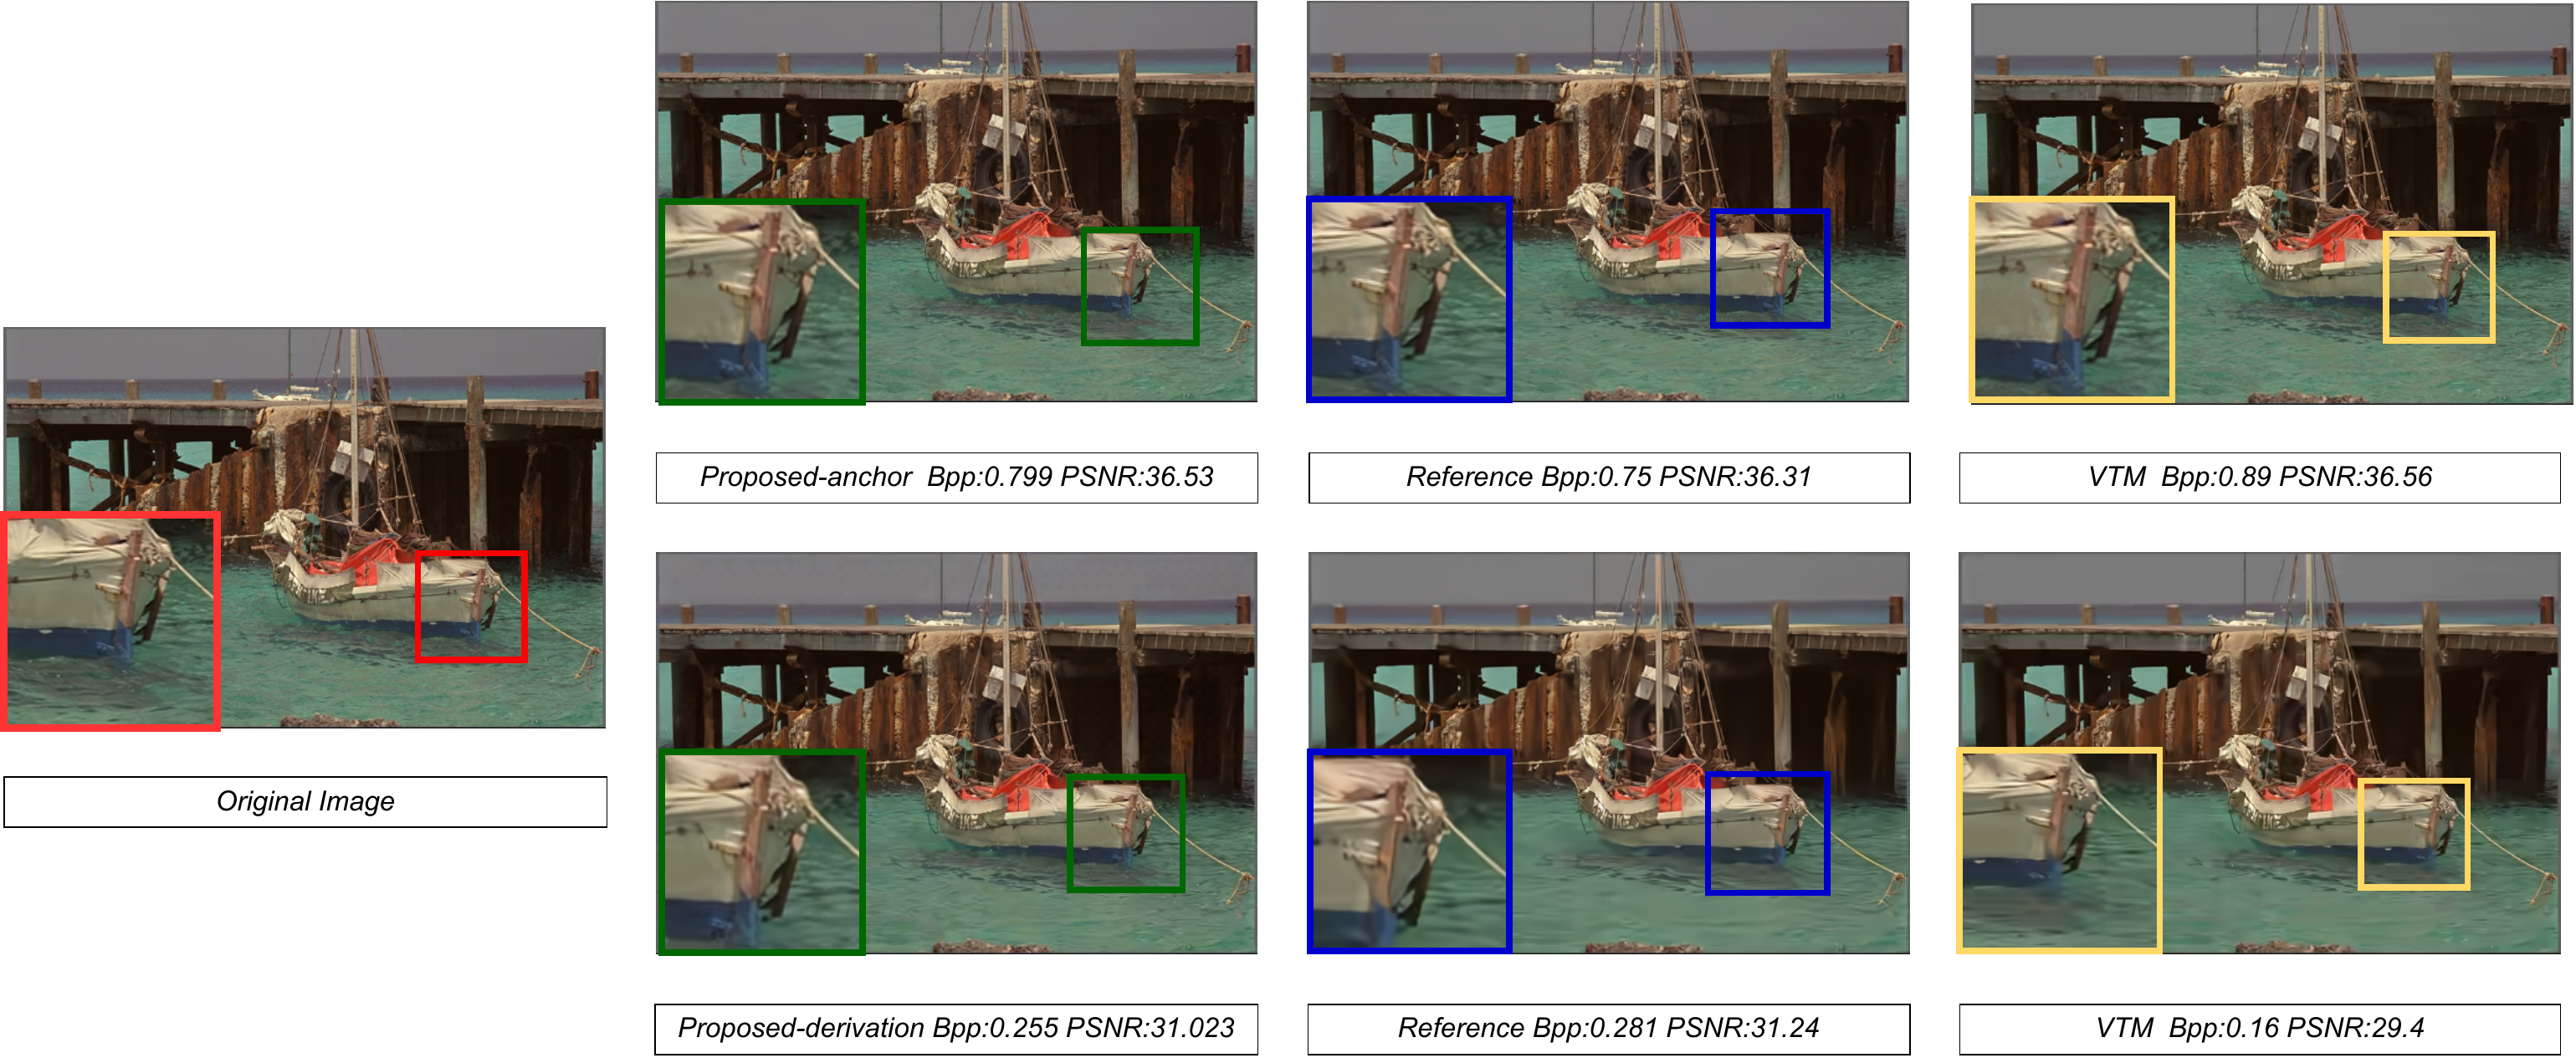}
 % \vspace{0.1cm}
  \caption{  Reconstruction of \emph{Kodim11} using \emph{Xie21} as reference. First row: Original image. Second Row: Comparison exploiting anchor model ($A_{1}$) Third Row: comparison exploiting Derivation model ($D_{21}$). Regarding reference, the closest one has been chosen. }
  \label{recostruct-xie}
%\end{minipage}
\end{figure*}

\begin{figure*}[h!]
%\begin{minipage}[b]{1.0\linewidth} 
  \centering
 \includegraphics[width=\textwidth]{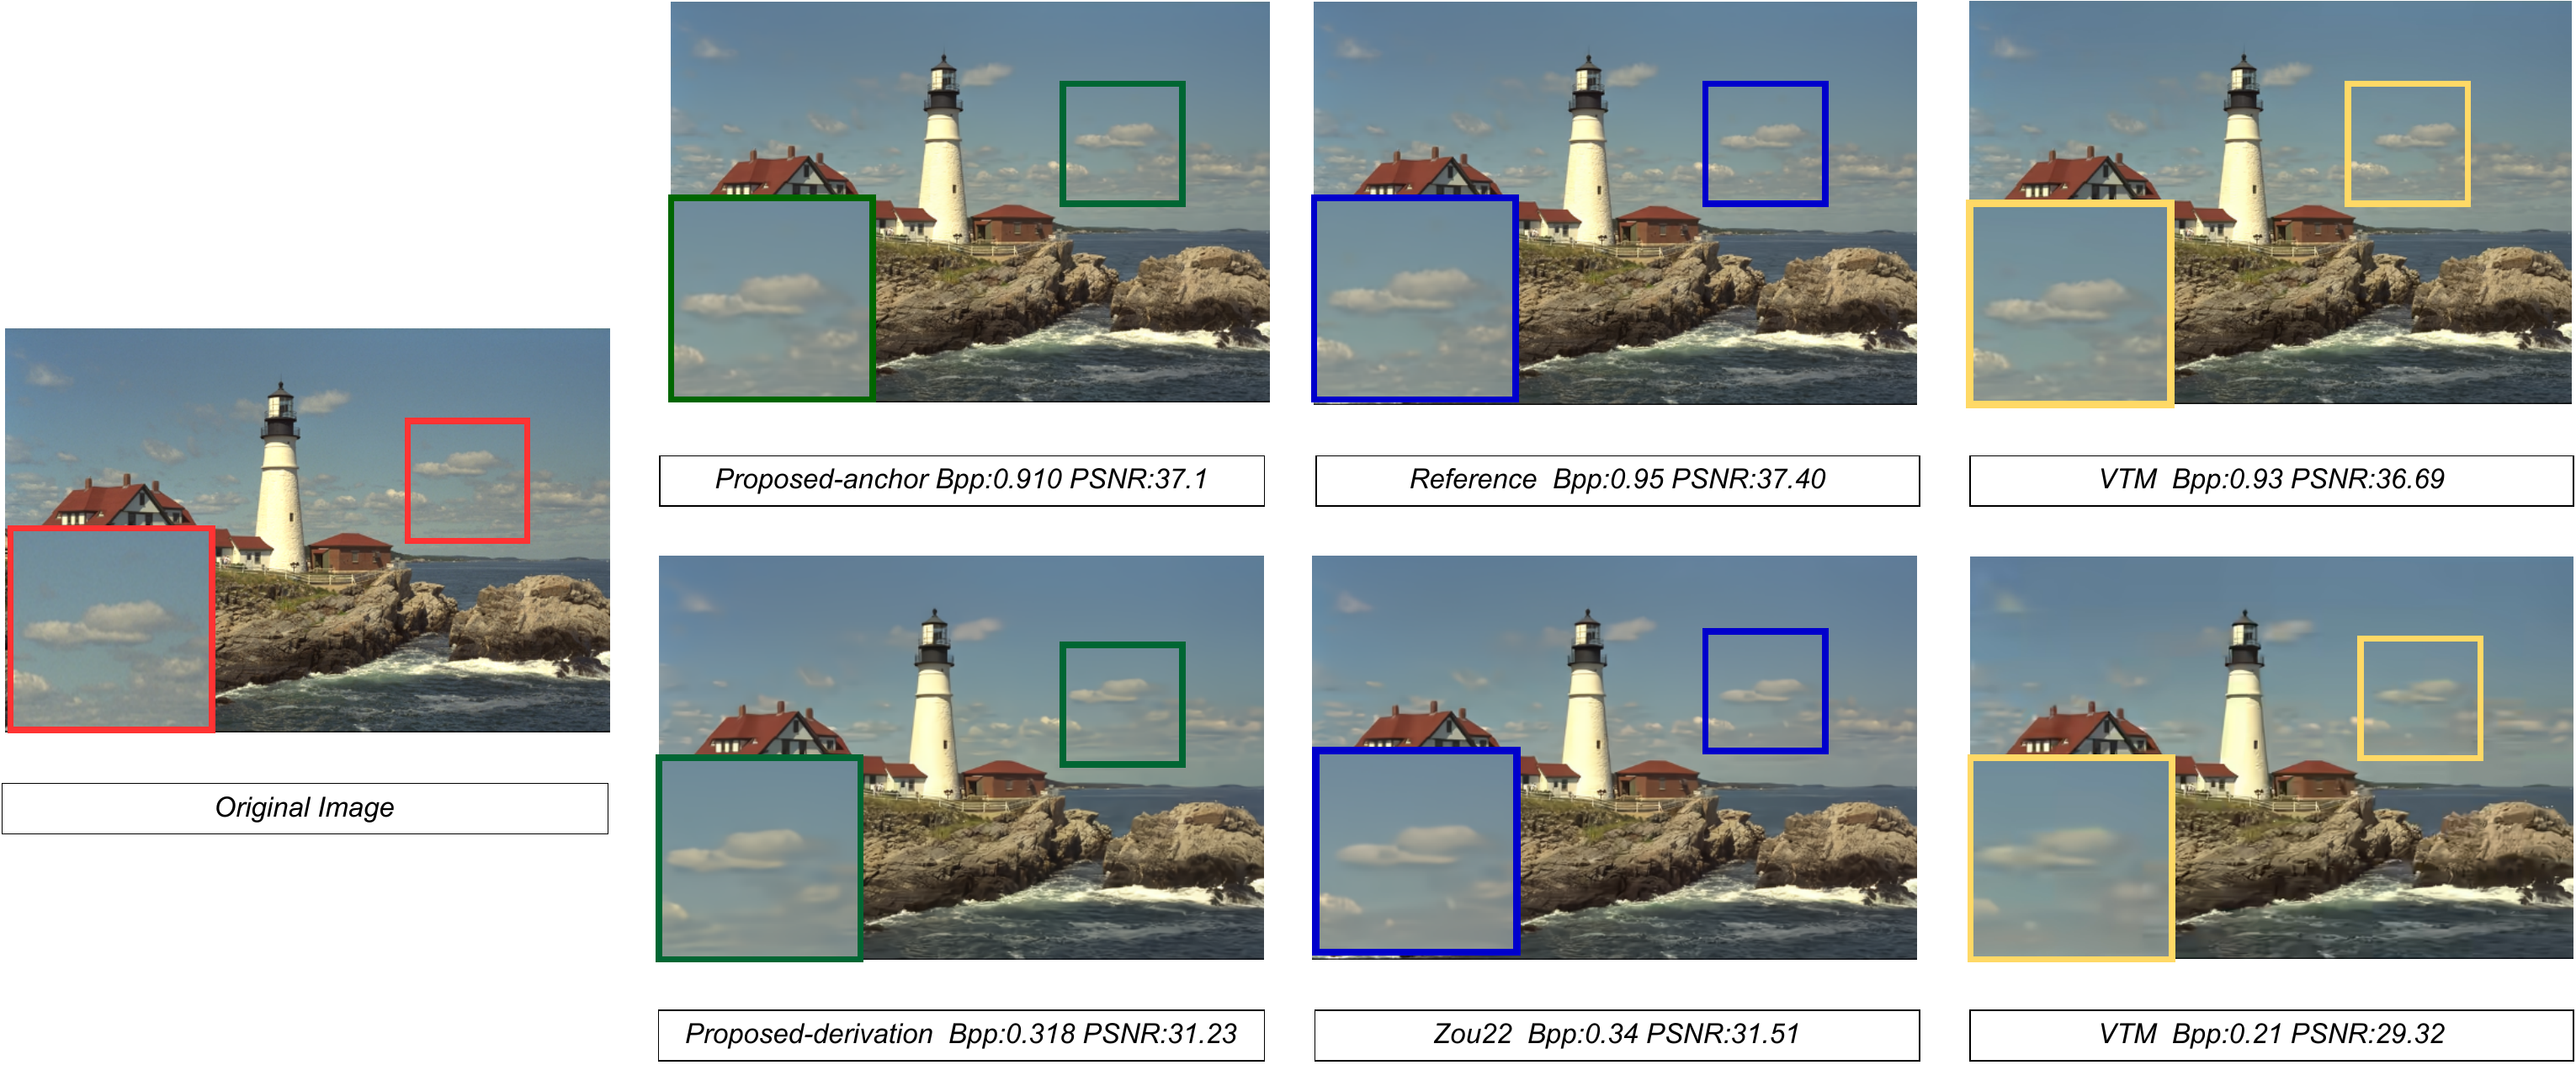}
 % \vspace{0.1cm}
  \caption{  Reconstruction of \emph{Kodim21} using \emph{Zou22} as reference. First row: Original image. Second Row: Comparison exploiting anchor model ($A_{1}$) Third Row: comparison exploiting Derivation model ($D_{21}$). Regarding reference, the closest one has been chosen. }
  \label{recostruct-zou}
%\end{minipage}
\end{figure*}
